# Supplementary material for: Molecular dynamics simulation analysis of structural dynamic cross correlation induced by odorant hydrogen-bonding in mouse eugenol olfactory receptor
Source: arXiv:2311.02654 ancillary file (2024-01-18)
Supplement: Supplementary file 1 [file sup03.pdf]

## Supplementary Materials on

### Molecular dynamics simulation analysis of structural dynamic cross correlation induced by odorant hydrogen-bonding in mouse eugenol olfactory receptor

Chisato Okamoto and Koji Ando

*Department of Information and Sciences, Tokyo Woman's Christian University, Tokyo 167-8585, Japan*

#### Supplementary Figure S1

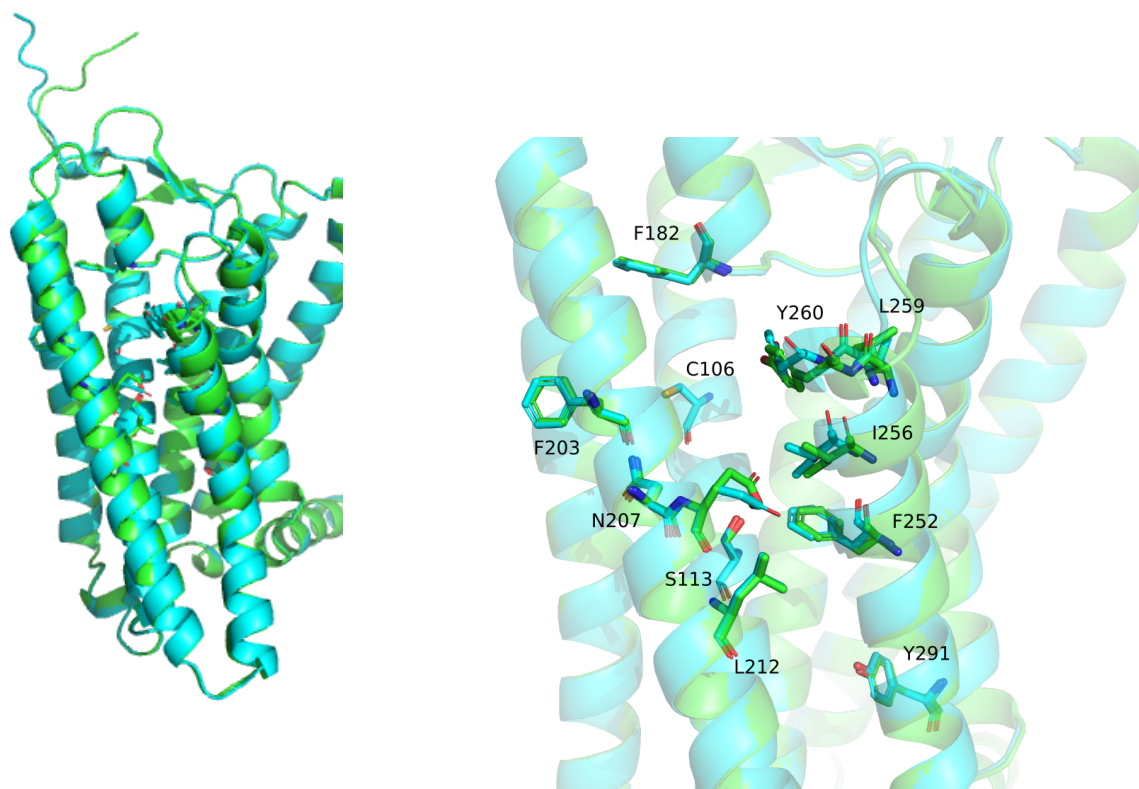

**Supplementary Figure S1** Comparison between the present result from the ColabFold server (green, accessed on July 8, 2022) and the UniProt entry Q920P2 (cyan, AF-Q920P2-F1-model\_v4.pdb). The right panel corresponds to Figure 1 in the main text.

## Supplementary Figure S2

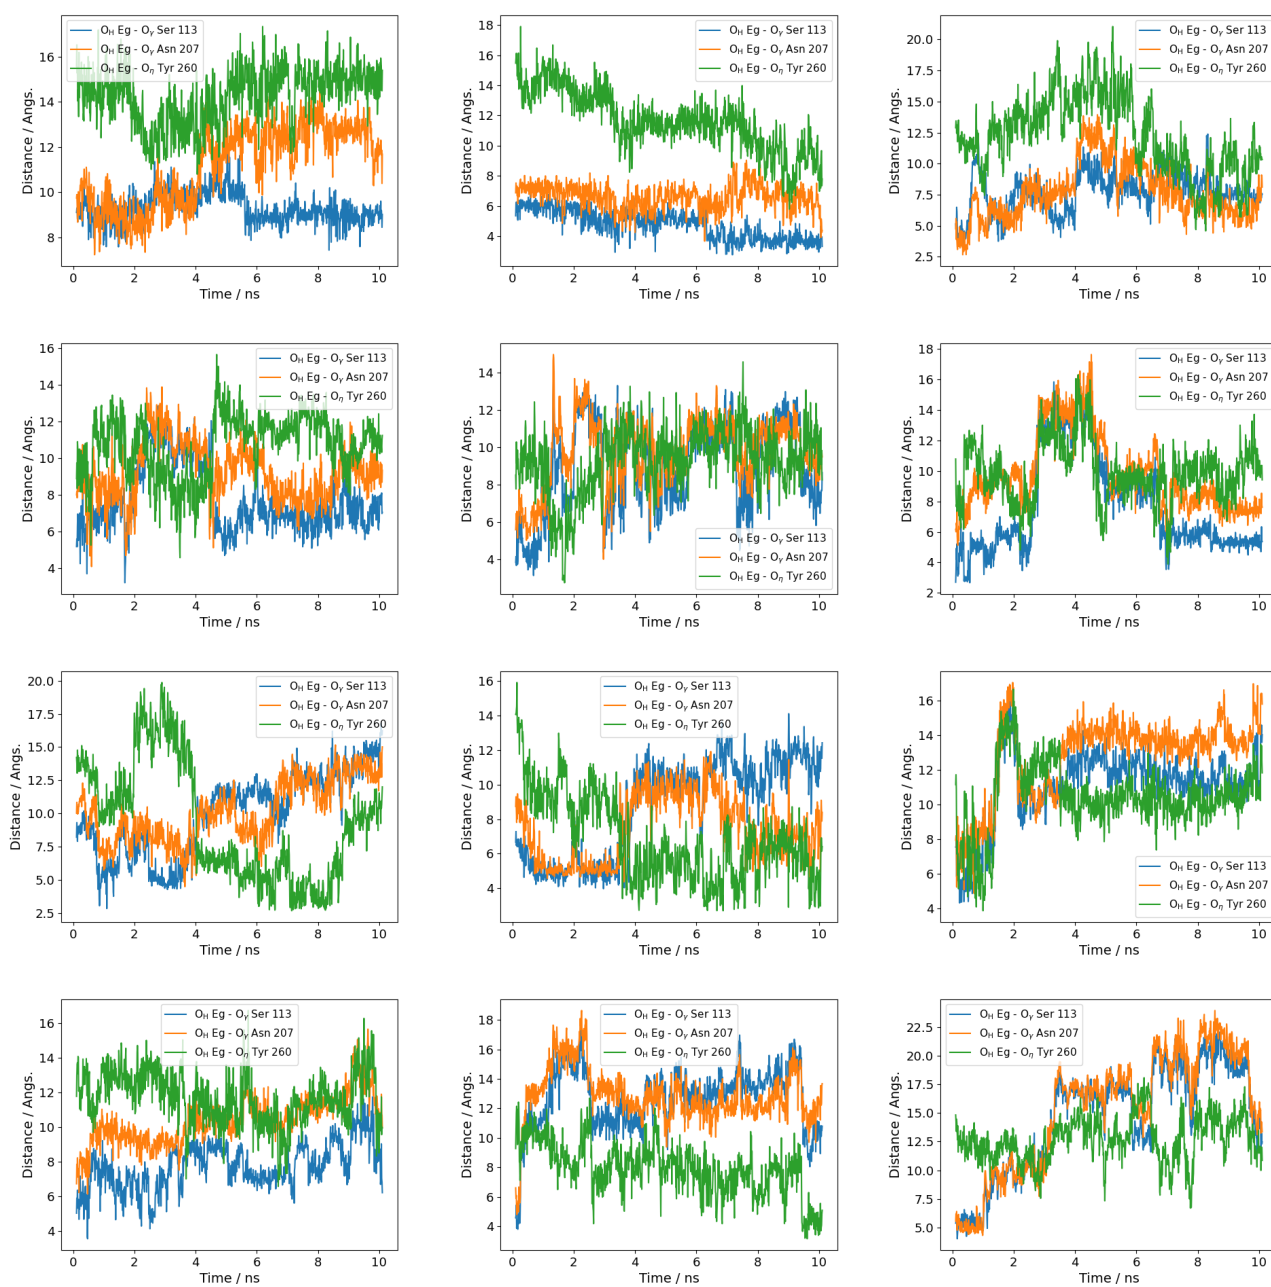

**Supplementary Figure S2** Eighteen trajectories (in addition to the two in Figure 3 in the main text) of the distance between O<sub>H</sub> atom of eugenol and O atoms of Ser113, Asn207, and Tyr260 starting from the docking configurations. (Continue to next page.)

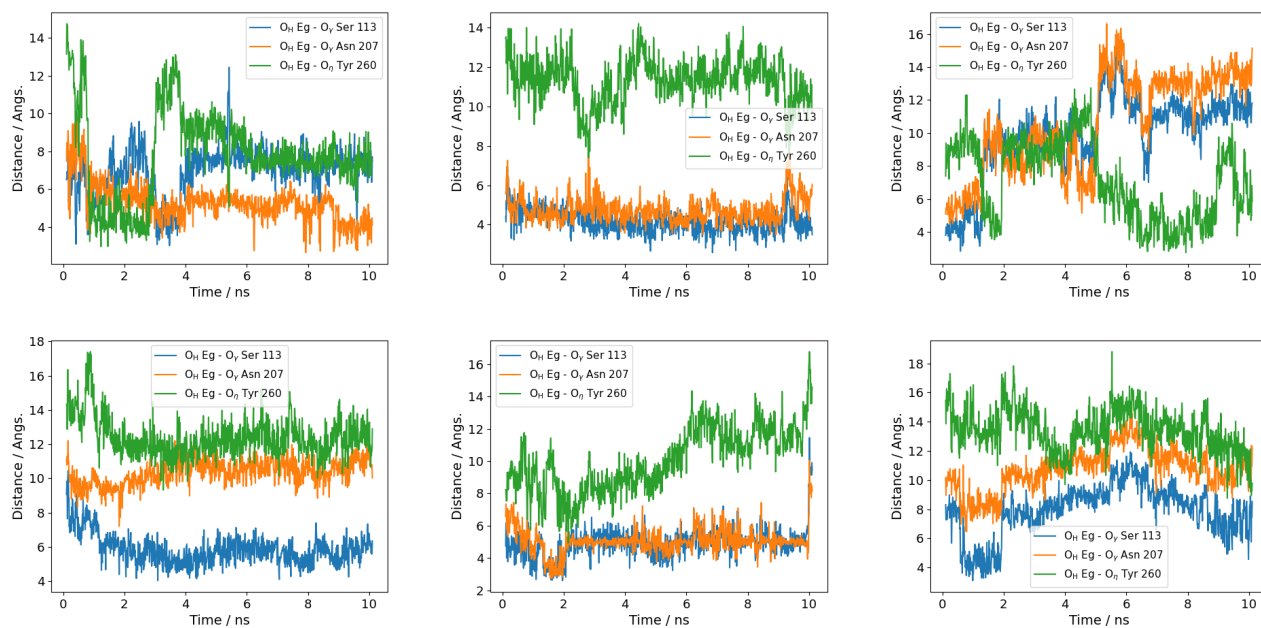

**Supplementary Figure S2 (conitued)**

### Supplementary Figure S3

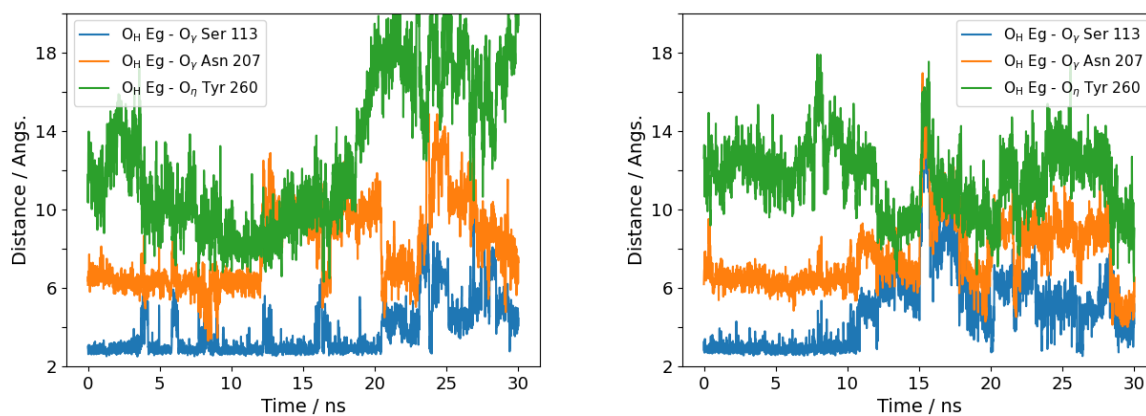

**Supplementary Figure S3** Two trajectories of the distance between  $O_H$  atom of eugenol and  $O$  atoms of Ser113, Asn207, and Tyr260 that maintained the eugenol-Ser113 hydrogen-bond for longer than 10 ns.

## Supplementary Figure S4

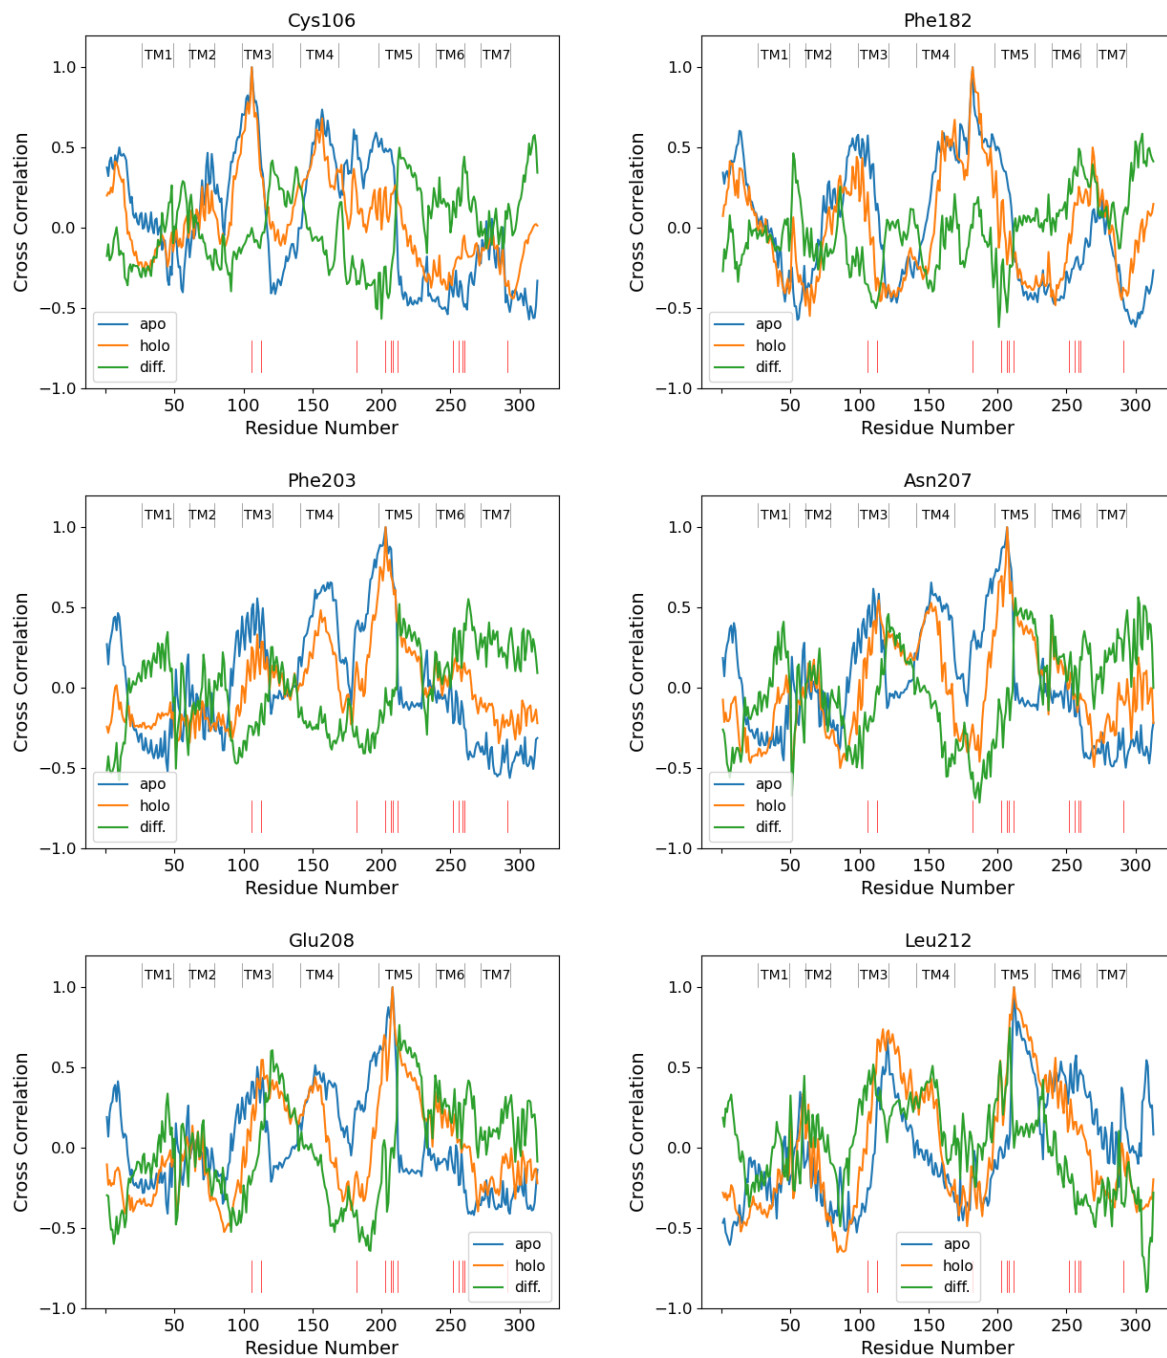

**Supplementary Figure S4** Sections of the dynamic cross-correlation maps (Figure 6 of the main text) at eleven key residues other than Ser113 displayed in Figure 7 (a) of the main text. (Continue to next page.)

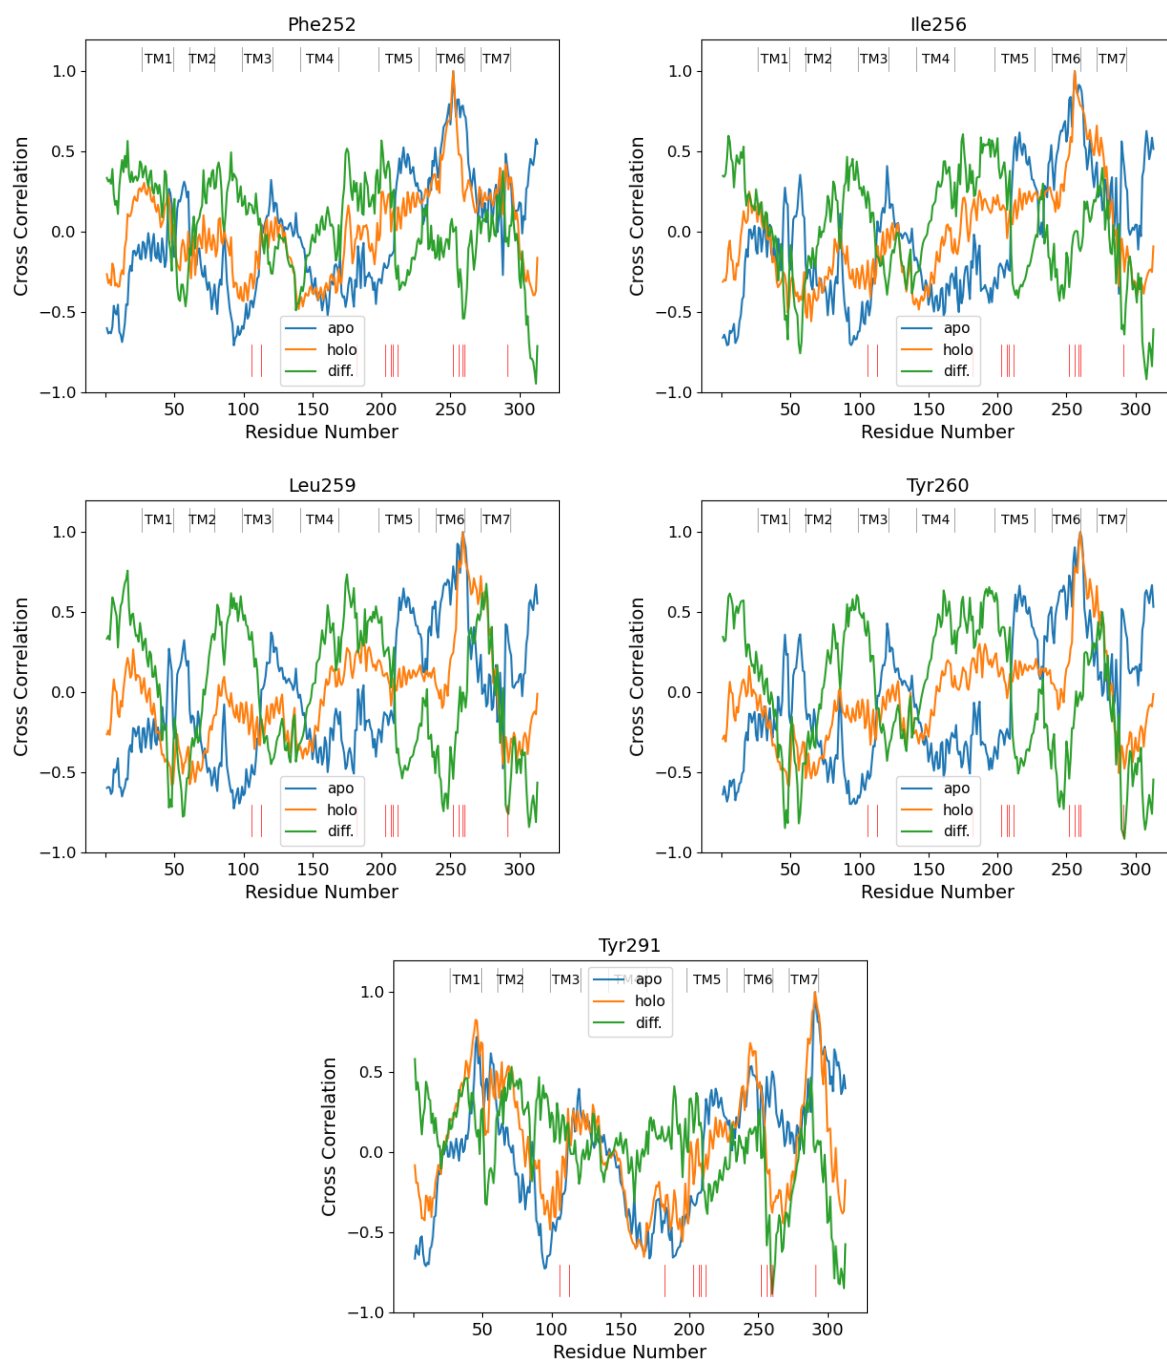

**Supplementary Figure S4** (continued)
